# Supplementary material for: SEAM: A Stochastic Benchmark for Multi-Document Tasks
Source: arXiv:2406.16086 source file (2024-06-23)
Supplement: Supplementary file 1 [file 11-SM.tex]

\newpage
\section{Datasheets for Datasets}
%%%%%%%%%%%%%%%%%%%%%%%%%%%%%%%%%%%%%%%%%%%%%%%%%%%%%%%%%%%%%%%%%%%%%%%%%%%%%%%%
\textbf{This document is based on \textit{Datasheets for Datasets} by Gebru et al. Please see the most updated version \underline{\textcolor{blue}{\href{http://arxiv.org/abs/1803.09010}{here}}}.}
%%%%%%%%%%%%%%%%%%%%%%%%%%%%%%%%%%%%%%%%%%%%%%%%%%%%%%%%%%%%%%%%%%%%%%%%%%%%%%%%
%\begin{mdframed}
\begin{mdframed}[linecolor=\sectioncolor]
\section*{\textcolor{\sectioncolor}{MOTIVATION
}}
\end{mdframed}

\textcolor{\sectioncolor}{\textbf{For what purpose was the dataset created?}
Was there a specific task in mind? Was there a specific gap that needed to be filled? Please provide a description.} \\
%%%
\name{} was created for two purposes: (1) standardize the evaluation of LLMs in \md{} tasks, and (2) to bridge the gap of the arbitrary choices taken when evaluating LLMs. For the former, we noticed that all popular LLM benchmarks consist of tasks that involve single-documents inputs, and there is no easy and standard way to evaluate \md{} tasks. For the latter, we noticed that many arbitrary choices that affect LLM performance needs to be taken when designing a benchmark, such as the instruction within the prompt, the order in which the documents are presented, and the few-shot examples given in the prompt. Instead of taking one arbitrary coice, we designed \name{} to sample over the space of arbitrary choices, and reported performance that take into account the variability of input/output.  \\

%%% 

\textcolor{\sectioncolor}{\textbf{Who created this dataset (e.g., which team, research group) and on behalf of which entity (e.g., company, institution, organization)?}} \\
    %%%
    This is an anonymous submission. We will update this information later. The team was led and supervised by an academic lab, without any corporate influence on the goals or presentation of any of the results.\\
    %%% 
    
    \textcolor{\sectioncolor}{\textbf{What support was needed to make this dataset?
    }
    (e.g.who funded the creation of the dataset? If there is an associated
    grant, provide the name of the grantor and the grant name and number, or if
    it was supported by a company or government agency, give those details.)
    } \\
    %%%
    To evaluate \name{} on SOTA LLMs, we needed computational power. We were supported by Google Research, who granted us with GCP credits for this project. Google did not affect or review any of the claims made in this paper.\\
    %%% 
    
    \textcolor{\sectioncolor}{\textbf{Any other comments?
    }} \\
    %%%
    No. \\
    %%%

%%%%%%%%%%%%%%%%%%%%%%%%%%%%%%%%%%%%%%%%%%%%%%%%%%%%%%%%%%%%%%%%%%%%%%%%%%%%%%%%
\begin{mdframed}[linecolor=\sectioncolor]
\section*{\textcolor{\sectioncolor}{COMPOSITION}}
\end{mdframed}
\textcolor{\sectioncolor}{\textbf{What do the instances that comprise the dataset represent (e.g., documents,
    photos, people, countries)?
    }
    Are there multiple types of instances (e.g., movies, users, and ratings;
    people and interactions between them; nodes and edges)? Please provide a
    description.
    } \\
    %%%
    \name{} consists of document text instances, from various domains. It includes news articles, reviews, Wikipedia pages, and scientific papers. \\
    %%% 
    
    \textcolor{\sectioncolor}{\textbf{How many instances are there in total (of each type, if appropriate)?
    }
    } \\
    %%%
    As detailed in Table~\ref{tab:datasets}, \name{} includes a total of 103K instances. For each domain: news - 57K, Wikipedia - 44K, reviews - 742, Scientific - 521. Since each instance involves multiple documents in its input, the total number of documents included in \name{} is much larger -- approximately 1.1M different documents. \\
    %\gabis{side note - do we actually have this 1.1M documents somewhere in the paper? I think it sounds impressive, we should probably mention it somehwere in abstract / intro.}  \\
    %%% 
    
    \textcolor{\sectioncolor}{\textbf{Does the dataset contain all possible instances or is it a sample (not
    necessarily random) of instances from a larger set?
    }
    If the dataset is a sample, then what is the larger set? Is the sample
    representative of the larger set (e.g., geographic coverage)? If so, please
    describe how this representativeness was validated/verified. If it is not
    representative of the larger set, please describe why not (e.g., to cover a
    more diverse range of instances, because instances were withheld or
    unavailable).
    } \\
    %%%
    \name{} consists of all instances from the original datasets. However, some labels from \musique{} and \fuse{} are not publicly available, thus we do not include instances without gold labels. Due to budget and computational constraints, it is not feasible to evaluate on the entire \name{} benchmark (though we provide such option in our code framework), so this paper we present the results over a randomly-sampled subset of \name{}. The random sampling process is done to each of the datasets separately, to ensure that all tasks and domains are covered and representing the complete dataset. It is up to the user choice wether to evaluate over the entire benchmark, or to randomly sample the number of instances that are feasible given their computational and budget constraints.  \\
    %%% 
    
    \textcolor{\sectioncolor}{\textbf{What data does each instance consist of?
    }
    “Raw” data (e.g., unprocessed text or images) or features? In either case,
    please provide a description.
    } \\
    %%%
    For \mn{}, \asp{} and \musique{} each instance consists of raw text. For \fuse{}, on top of the raw text we add highlight markers within the text (as done in the original paper), to mark the spans of which the model is expected to fuse information from. For \ecb{} and \scico{}, we mark each entity or event mention in the text with `[mention](id)', so that the model is expected to perform the linking between coreferring mentions, based on the ids we provide. In addition, for each input instance we combine a specific task instruction, and 3-shot examples, as shown in Figure~\ref{fig:prompt-template}. \\
    %%% 
    
    \textcolor{\sectioncolor}{\textbf{Is there a label or target associated with each instance?
    }
    If so, please provide a description.
    } \\
    %%%
    Yes. For summarization datasets there is a reference summary for each instance. For question answering, there is a boolean that holds wether the answer can be deduced from the provided documents, and the answer to the question. For the coreference datasets, the list of gold clusters are provided, where each cluster is a list of mention ids belong to the cluster. \\
    %%% 
    
    \textcolor{\sectioncolor}{\textbf{Is any information missing from individual instances?
    }
    If so, please provide a description, explaining why this information is
    missing (e.g., because it was unavailable). This does not include
    intentionally removed information, but might include, e.g., redacted text.
    } \\
    %%%
    Yes. \fuse{} and \musique{} does not provide gold labels for their test split, so we do not include these instances in \name{}. \\
    %%% 
    
    \textcolor{\sectioncolor}{\textbf{Are relationships between individual instances made explicit (e.g., users’
    movie ratings, social network links)?
    }
    If so, please describe how these relationships are made explicit.
    } \\
    %%%
    No. The linking is \textit{within} each individual instances, e.g., each individual instance in \fuse{} consists of 8 reviews from different people to the same product/service. No explicit relationships \textit{across} instance. \\
    %%% 
    
    \textcolor{\sectioncolor}{\textbf{Are there recommended data splits (e.g., training, development/validation,
    testing)?
    }
    If so, please provide a description of these splits, explaining the
    rationale behind them.
    } \\
    %%%
    The original datasets included in \name{} provide train/validation/test splits, but since \name{} is intended to evaluate LLMs in inference time, and training is not feasible for such massive models, we do not keep these split as an inherent part of \name{}. But, when sampling an instance of \name{}, the user can specify from which split they want to sample, based on the original train/validation/test splits.  \\
    %%% 
    
    \textcolor{\sectioncolor}{\textbf{Are there any errors, sources of noise, or redundancies in the dataset?
    }
    If so, please provide a description.
    } \\
    %%%
    We use previously-curated datasets which may contain errors and noise within their gold labels, for example in the reference summaries provided with the summarization datasets. But, we do not add any new instances that affect the previously-curated errors and noise. \\
    % Beyond the errors and noise that may appear in the original datasets, the curation of \name{} may have injected additional noise and errors. \gabis{I would actually stop here and say that we use the original datasets and they may contain errors, but that we don't add any new instances. I don't think that what follows here is related to the question (e.g., if the question appears before or after the prompt may lead the models to err, but that's not related to errors in the datasets IMO.}
    
    % As mentioned in the paper, LLMs are sensitive to variations in prompts, thus we suggest to sample over the space of arbitrary choices. However, we do not cover the entire space of options: (1) we relaxed the infinite space of instruction-paraphrasing possibilities, to a finite set of 20 paraphrases for each dataset. (2) For \musique{}, we provide the question \textit{before} the documents, which may yield different results from showing it \textit{after} the documents. (3) For the coreference datasets, we decide on one specific format for mentions marking. (3) For \fuse{}, we go with one specific format for highlight markers. (4) For QA and coreference tasks, which require a structured output format, we expected a specific JSON format for the output. (5) We have a single prompt template as presented in Figure~\ref{fig:prompt-template}. All of the above add noise to the reported results, and in future work we can add more axis to sample above, to reduce such noise.  \\
    %%% 
    
    \textcolor{\sectioncolor}{\textbf{Is the dataset self-contained, or does it link to or otherwise rely on
    external resources (e.g., websites, tweets, other datasets)?
    }
    If it links to or relies on external resources, a) are there guarantees
    that they will exist, and remain constant, over time; b) are there official
    archival versions of the complete dataset (i.e., including the external
    resources as they existed at the time the dataset was created); c) are
    there any restrictions (e.g., licenses, fees) associated with any of the
    external resources that might apply to a future user? Please provide
    descriptions of all external resources and any restrictions associated with
    them, as well as links or other access points, as appropriate.
    } \\
    %%%
    \name{} is self-contained. \\
    %%% 
    
    \textcolor{\sectioncolor}{\textbf{Does the dataset contain data that might be considered confidential (e.g.,
    data that is protected by legal privilege or by doctor-patient
    confidentiality, data that includes the content of individuals’ non-public
    communications)?
    }
    If so, please provide a description.
    } \\
    %%%
    No. However, the data in \asp{}, which is based on the DUC dataset, requires access rights from NIST (the curators of DUC). \\
    %%% 
    
    \textcolor{\sectioncolor}{\textbf{Does the dataset contain data that, if viewed directly, might be offensive,
    insulting, threatening, or might otherwise cause anxiety?
    }
    If so, please describe why.
    } \\
    %%%
    No.  \\
    %%% 
    
    \textcolor{\sectioncolor}{\textbf{Does the dataset relate to people?
    }
    If not, you may skip the remaining questions in this section.
    } \\
    %%%
    Yes, e.g., people that are mentioned in news articles or Wikipedia pages. However, all of the data is in the public domain and we did not collect any additional personal information about people. \\
    %\gabis{I don't think this is what the question asks, I think that they mean if real-world people are mentioned in it. I still think that the answer is yes, because it has e.g., news. But I would say here that all of the data is in the public domain anyway and we didn't collect any additional personal information about people.}\\
    %%% 
    
    \textcolor{\sectioncolor}{\textbf{Does the dataset identify any subpopulations (e.g., by age, gender)?
    }
    If so, please describe how these subpopulations are identified and
    provide a description of their respective distributions within the dataset.
    } \\
    %%%
    No. This information is not provided within the data. \\
    %%% 
    
    \textcolor{\sectioncolor}{\textbf{Is it possible to identify individuals (i.e., one or more natural persons),
    either directly or indirectly (i.e., in combination with other data) from
    the dataset?
    }
    If so, please describe how.
    } \\
    %%%
    Yes, as we deal with news reports which contain references to real-world events and entities. But these are all in the public domain, and we didn't collect any new texts in this work.\\
    %%% 
    
    \textcolor{\sectioncolor}{\textbf{Does the dataset contain data that might be considered sensitive in any way
    (e.g., data that reveals racial or ethnic origins, sexual orientations,
    religious beliefs, political opinions or union memberships, or locations;
    financial or health data; biometric or genetic data; forms of government
    identification, such as social security numbers; criminal history)?
    }
    If so, please provide a description.
    } \\
    %%%
    No. \\
    %%% 
    
    \textcolor{\sectioncolor}{\textbf{Any other comments?
    }} \\
    %%%
    No. \\
    %%%

%%%%%%%%%%%%%%%%%%%%%%%%%%%%%%%%%%%%%%%%%%%%%%%%%%%%%%%%%%%%%%%%%%%%%%%%%%%%%%%%
\begin{mdframed}[linecolor=\sectioncolor]
\section*{\textcolor{\sectioncolor}{COLLECTION
}}
\end{mdframed}

    \textcolor{\sectioncolor}{\textbf{How was the data associated with each instance acquired?
    }
    Was the data directly observable (e.g., raw text, movie ratings),
    reported by subjects (e.g., survey responses), or indirectly
    inferred/derived from other data (e.g., part-of-speech tags, model-based
    guesses for age or language)? If data was reported by subjects or
    indirectly inferred/derived from other data, was the data
    validated/verified? If so, please describe how.
    } \\
    %%%
    The data in \name{} is directly observable, as it consists of raw texts.  \\
    %%% 
    
    \textcolor{\sectioncolor}{\textbf{Over what timeframe was the data collected?
    }
    Does this timeframe match the creation timeframe of the data associated
    with the instances (e.g., recent crawl of old news articles)? If not,
    please describe the timeframe in which the data associated with the
    instances was created. Finally, list when the dataset was first published.
    } \\
    %%%
    Our dataset does not contain any new data collection. We cite the relevant work for further details on how they were collected. \\
    % Each dataset in \name{} was published in different time. Datasets in NLP do not usually describe the timeframe in which the documents were collected (e.g., when was a review was written or a news article was published), but we assume that they were relevant to the time that the dataset was published. \mn{} was published in 2019. \asp{} is based on \mn{} and DUC, where the news articles from DUC are from 2001, 2002, 2006 and 2007. \fuse{} consists of business reviews from previously published papers, which were originally presented in 2016. \ecb{} is a dataset from 2012, which is based on ECB from 2010. \scico{} uses scientific papers from previously published datasets from 2019 and 2020. \musique{} composes single-hop questions from papers that were published in 2016-2020. The Wikipedia pages that are used as evidence are not provided with information regarding when they were created.     \\
    %%% 
    
    \textcolor{\sectioncolor}{\textbf{What mechanisms or procedures were used to collect the data (e.g., hardware
    apparatus or sensor, manual human curation, software program, software
    API)?
    }
    How were these mechanisms or procedures validated?
    } \\
    %%%
    Our dataset doesn't contain any new data collection. We cite the relevant work for further details on how they were collected. \\
    % The evidence documents were crawled from the internet. The reference summaries for the summarization datasets were manually human created via a diverse set pf protocols, detailed for each different dataset in its original paper. The coreference gold clusters were also annotated but humans, using popular coreference annotation protocols. The answers for the multi-hop questions were composed from the single-hop decomposition answers.  \\
    %%% 
    
    \textcolor{\sectioncolor}{\textbf{What was the resource cost of collecting the data?
    }
    (e.g. what were the required computational resources, and the associated
    financial costs, and energy consumption - estimate the carbon footprint.
    See Strubell et al. for approaches in this area.)
    } \\
    %%%
    \name{} includes already-existing datasets, so we had no additional costs. \\
    %%% 
    
    \textcolor{\sectioncolor}{\textbf{If the dataset is a sample from a larger set, what was the sampling
    strategy (e.g., deterministic, probabilistic with specific sampling
    probabilities)?
    }
    } \\
    %%%
    We include all instances from original datasets. However, if a user wants to evaluate its dataset on a smaller set, we allow a random sampling. \\
    %%% 
    
    \textcolor{\sectioncolor}{\textbf{Who was involved in the data collection process (e.g., students,
    crowdworkers, contractors) and how were they compensated (e.g., how much
    were crowdworkers paid)?
    }
    } \\
    %%%
    \name{} includes already-existing datasets, so the data collection process only involved our research group. \\
    %%% 
    
    \textcolor{\sectioncolor}{\textbf{Were any ethical review processes conducted (e.g., by an institutional
    review board)?
    }
    If so, please provide a description of these review processes, including
    the outcomes, as well as a link or other access point to any supporting
    documentation.
    } \\
    %%%
    Our dataset does not contain any new data collection. The leading author is certified with CITI program course~\href{https://about.citiprogram.org/course/human-subjects-research-social-behavioral-educational-sbe-refresher-1/}{“Social \& Behavioral Research - Basic/Refresher”}, following the research institution’s requirements.  \\
    %%% 
    
    \textcolor{\sectioncolor}{\textbf{Does the dataset relate to people?
    }
    If not, you may skip the remainder of the questions in this section.
    } \\
    %%%
    No. \\
    %%% 
    
    \textcolor{\sectioncolor}{\textbf{Did you collect the data from the individuals in question directly, or
    obtain it via third parties or other sources (e.g., websites)?
    }
    } \\
    %%%
    Irrelevant. \\
    %%% 
    
    \textcolor{\sectioncolor}{\textbf{Were the individuals in question notified about the data collection?
    }
    If so, please describe (or show with screenshots or other information) how
    notice was provided, and provide a link or other access point to, or
    otherwise reproduce, the exact language of the notification itself.
    } \\
    %%%
    Irrelevant. \\
    %%% 
    
    \textcolor{\sectioncolor}{\textbf{Did the individuals in question consent to the collection and use of their
    data?
    }
    If so, please describe (or show with screenshots or other information) how
    consent was requested and provided, and provide a link or other access
    point to, or otherwise reproduce, the exact language to which the
    individuals consented.
    } \\
    %%%
    Irrelevant. \\
    %%% 
    
    \textcolor{\sectioncolor}{\textbf{If consent was obtained, were the consenting individuals provided with a
    mechanism to revoke their consent in the future or for certain uses?
    }
     If so, please provide a description, as well as a link or other access
     point to the mechanism (if appropriate)
    } \\
    %%%
    Irrelevant. \\
    %%% 
    
    \textcolor{\sectioncolor}{\textbf{Has an analysis of the potential impact of the dataset and its use on data
    subjects (e.g., a data protection impact analysis)been conducted?
    }
    If so, please provide a description of this analysis, including the
    outcomes, as well as a link or other access point to any supporting
    documentation.
    } \\
    %%%
    Irrelevant. \\
    %%% 
    
    \textcolor{\sectioncolor}{\textbf{Any other comments?
    }} \\
    %%%
    No. \\
    %%%

%%%%%%%%%%%%%%%%%%%%%%%%%%%%%%%%%%%%%%%%%%%%%%%%%%%%%%%%%%%%%%%%%%%%%%%%%%%%%%%%
\begin{mdframed}[linecolor=\sectioncolor]
\section*{\textcolor{\sectioncolor}{
    PREPROCESSING / CLEANING / LABELING
}}
\end{mdframed}

    \textcolor{\sectioncolor}{\textbf{Was any preprocessing/cleaning/labeling of the data
    done(e.g.,discretization or bucketing, tokenization, part-of-speech
    tagging, SIFT feature extraction, removal of instances, processing of
    missing values)?
    }
    If so, please provide a description. If not, you may skip the remainder of
    the questions in this section.
    } \\
    %%%
    For the coreference dataset, we pre-processed each document by marking the annotated entity or event mention. For \fuse{} we add highlight markers to spans of text that the model is expected to fuse information from. We also prepare the input prompt for the model, by combining an instruction for the specific task, 3-shot examples, and the instance itself (i.e., evidence documents). \\
    %%%

    \textcolor{\sectioncolor}{\textbf{Was the “raw” data saved in addition to the preprocessed/cleaned/labeled
    data (e.g., to support unanticipated future uses)?
    }
    If so, please provide a link or other access point to the “raw” data.
    } \\
    %%%
    Yes. we save also the original documents in addition to the processed input prompt. \\
    %%%

    \textcolor{\sectioncolor}{\textbf{Is the software used to preprocess/clean/label the instances available?
    }
    If so, please provide a link or other access point.
    } \\
    %%%
    Yes. It can be found in the project github.\footnote{\label{github}\url{https://github.com/seam-benchmark/SEAM}} \\
    %%%

    \textcolor{\sectioncolor}{\textbf{Any other comments?
    }} \\
    %%%
    No. \\
    %%%

%%%%%%%%%%%%%%%%%%%%%%%%%%%%%%%%%%%%%%%%%%%%%%%%%%%%%%%%%%%%%%%%%%%%%%%%%%%%%%%%
\begin{mdframed}[linecolor=\sectioncolor]
\section*{\textcolor{\sectioncolor}{
    USES
}}
\end{mdframed}

    \textcolor{\sectioncolor}{\textbf{Has the dataset been used for any tasks already?
    }
    If so, please provide a description.
    } \\
    %%%
    In the paper, we use \name{} to evaluate SOTA open-source LLMs.  \\
    %%%

    \textcolor{\sectioncolor}{\textbf{Is there a repository that links to any or all papers or systems that use the dataset?
    }
    If so, please provide a link or other access point.
    } \\
    %%%
    Yes. In our website we invite anyone who evaluates their model on \name{}, to contribute to the leaderboard we posted on our website.\footnote{\label{website}\url{https://seam-benchmark.github.io}} \\
    %%%

    \textcolor{\sectioncolor}{\textbf{What (other) tasks could the dataset be used for?
    }
    } \\
    %%%
    \name{} is intended to be used for LLMs evaluation.  \\
    %%%

    \textcolor{\sectioncolor}{\textbf{Is there anything about the composition of the dataset or the way it was
    collected and preprocessed/cleaned/labeled that might impact future uses?
    }
    For example, is there anything that a future user might need to know to
    avoid uses that could result in unfair treatment of individuals or groups
    (e.g., stereotyping, quality of service issues) or other undesirable harms
    (e.g., financial harms, legal risks) If so, please provide a description.
    Is there anything a future user could do to mitigate these undesirable
    harms?
    } \\
    %%%
    No. \\
    %%%

    \textcolor{\sectioncolor}{\textbf{Are there tasks for which the dataset should not be used?
    }
    If so, please provide a description.
    } \\
    %%%
    A misuse would be to include it in future LLMs, which will then make it unusable for evaluation. However, since we suggest a benchmark generator and not one static version, we can always come up with new instruction paraphrase or few-shot examples, and evaluate LLMs on ibnstances they did not see before. \\
    %%%

    \textcolor{\sectioncolor}{\textbf{Any other comments?
    }} \\
    %%%
    No. \\
    %%%

%%%%%%%%%%%%%%%%%%%%%%%%%%%%%%%%%%%%%%%%%%%%%%%%%%%%%%%%%%%%%%%%%%%%%%%%%%%%%%%%
\begin{mdframed}[linecolor=\sectioncolor]
\section*{\textcolor{\sectioncolor}{
    DISTRIBUTION
}}
\end{mdframed}

    \textcolor{\sectioncolor}{\textbf{Will the dataset be distributed to third parties outside of the entity
    (e.g., company, institution, organization) on behalf of which the dataset
    was created?
    }
    If so, please provide a description.
    } \\
    %%%
    %\gabis{I don't understand the question. I'm not sure if they expect us to answer ``Yes'' It's public, right? so anyone can use it. Maybe let's write ``.'' and let the readr understand whatever they want from this?}
    The dataset is made publicly available for public use. \\
    %%%

    \textcolor{\sectioncolor}{\textbf{How will the dataset will be distributed (e.g., tarball on website, API,
    GitHub)?
    }
    Does the dataset have a digital object identifier (DOI)?
    } \\
    %%%
    We provide a project website\footref{website}, github repository\footref{github} and a zip file containing the data\footnote{\url{https://drive.google.com/file/d/1H6pBzwJmCfFGOWOOzyLDFID2lIk9bbfI/view}}. \\
    %%%

    \textcolor{\sectioncolor}{\textbf{When will the dataset be distributed?
    }
    } \\
    %%%
    It is already distributed (June 2024). \\
    %%%

    \textcolor{\sectioncolor}{\textbf{Will the dataset be distributed under a copyright or other intellectual
    property (IP) license, and/or under applicable terms of use (ToU)?
    }
    If so, please describe this license and/or ToU, and provide a link or other
    access point to, or otherwise reproduce, any relevant licensing terms or
    ToU, as well as any fees associated with these restrictions.
    } \\
    %%%
    The dataset is distributed under Apache 2.0 license. \\
    %%%

    \textcolor{\sectioncolor}{\textbf{Have any third parties imposed IP-based or other restrictions on the data
    associated with the instances?
    }
    If so, please describe these restrictions, and provide a link or other
    access point to, or otherwise reproduce, any relevant licensing terms, as
    well as any fees associated with these restrictions.
    } \\
    %%%
    For using the data based DUC, access should be granted from NIST.\footnote{\url{https://duc.nist.gov}}  \\
    %%%

    \textcolor{\sectioncolor}{\textbf{Do any export controls or other regulatory restrictions apply to the
    dataset or to individual instances?
    }
    If so, please describe these restrictions, and provide a link or other
    access point to, or otherwise reproduce, any supporting documentation.
    } \\
    %%%
    We restrict the use of \name{} as part of the training set of future LLMs. \\
    %%%

    \textcolor{\sectioncolor}{\textbf{Any other comments?
    }} \\
    %%%
    No. \\
    %%%

%%%%%%%%%%%%%%%%%%%%%%%%%%%%%%%%%%%%%%%%%%%%%%%%%%%%%%%%%%%%%%%%%%%%%%%%%%%%%%%%
\begin{mdframed}[linecolor=\sectioncolor]
\section*{\textcolor{\sectioncolor}{MAINTENANCE
}}
\end{mdframed}

    \textcolor{\sectioncolor}{\textbf{Who is supporting/hosting/maintaining the dataset?
    }
    } \\
    %%%
    This is an anonymous submission, we will provide further details after the review process. \\
    %%%

    \textcolor{\sectioncolor}{\textbf{How can the owner/curator/manager of the dataset be contacted (e.g., email
    address)?
    }
    } \\
    %%%
    Email the \name-benchmark group via \href{mailto:seam.benchmark@gmail.com}{seam.benchmark@gmail.com}. \\
    %%%

    \textcolor{\sectioncolor}{\textbf{Is there an erratum?
    }
    If so, please provide a link or other access point.
    } \\
    %%%
    No. \\
    %%%

    \textcolor{\sectioncolor}{\textbf{Will the dataset be updated (e.g., to correct labeling errors, add new
    instances, delete instances)?
    }
    If so, please describe how often, by whom, and how updates will be
    communicated to users (e.g., mailing list, GitHub)?
    } \\
    %%%
    Yes. \name{} is intended to be constantly updated, including new \md{} datasets and tasks that will come out, and omitting datasets if they are no longer relevant. We will communicate the updates via our website and github repository.  \\
    %%%

    \textcolor{\sectioncolor}{\textbf{If the dataset relates to people, are there applicable limits on the
    retention of the data associated with the instances (e.g., were individuals
    in question told that their data would be retained for a fixed period of
    time and then deleted)?
    }
    If so, please describe these limits and explain how they will be enforced.
    } \\
    %%%
    Irrelevant. \\
    %%%

    \textcolor{\sectioncolor}{\textbf{Will older versions of the dataset continue to be
    supported/hosted/maintained?
    }
    If so, please describe how. If not, please describe how its obsolescence
    will be communicated to users.
    } \\
    %%%
    Yes. Users will be able to configure the dataset generation based on the dataset version they wish to include. \\
    %%%

    \textcolor{\sectioncolor}{\textbf{If others want to extend/augment/build on/contribute to the dataset, is
    there a mechanism for them to do so?
    }
    If so, please provide a description. Will these contributions be
    validated/verified? If so, please describe how. If not, why not? Is there a
    process for communicating/distributing these contributions to other users?
    If so, please provide a description.
    } \\
    %%%
    Yes. In our github repository we provide detailed information on how to add new datasets and how to evaluate new models on \name{}. \\
    %%%

    \textcolor{\sectioncolor}{\textbf{Any other comments?
    }} \\
    %%%
    No. \\
    %%%
